# Supplementary material for: Learning to read residual images for single-pixel photography
Source: arXiv:2611.03729 source file (2026-11-01)
Supplement: Supplementary file 1 [file supplementary.tex]

\clearpage
\section*{Supplementary information}
\setcounter{figure}{0}
\renewcommand{\thefigure}{S\arabic{figure}}

\bmhead{Supplementary videos}
The rolling reconstructions of Fig.~\ref{fig:video} are provided as videos at the native frame rate of each clip, one per method together with a side-by-side video of the ground truth, Measurement-Gradient-Conditioned Video Flow (MGV-Flow), history-conditioned flow matching (History-FM) and FlowDPS-inspired, for the factory floor, touchdown pass and speed bag clips.
